# Supplementary material for: Embedded SML using the MLton compiler
Source: arXiv:1608.07206 source file (2016-08-25)
Supplement: Supplementary file 1 [file appendix.tex]

This is the text of the appendix, if you need one.
